# Supplementary material for: EOM-CC Methods with Approximate Triple Excitations for NEXAFS and XPS
Source: arXiv:2001.09218 ancillary file (2020-01-24)
Supplement: Supplementary file 1 [file si.pdf]

# EOM-CC Methods with Approximate Triple Excitations for NEXAFS and XPS: Supplemental Information

Devin A. Matthews*

Southern Methodist University, Dallas, TX 75275

**ARTICLE HISTORY**
Compiled January 24, 2020

## 1. Molecular Geometries

$C_2H_4$ (a.u.):

| | | | |
|---|---|---|---|
| C | −1.25732954 | 0 | 0 |
| C | 1.25732954 | 0 | 0 |
| H | −2.32276354 | 1.74272408 | 0 |
| H | −2.32276354 | −1.74272408 | 0 |
| H | 2.32276354 | 1.74272408 | 0 |
| H | 2.32276354 | −1.74272408 | 0 |

HCN (Å):

| | | | |
|---|---|---|---|
| H | 0 | 0 | 1.068 |
| C | 0 | 0 | 0 |
| N | 0 | 0 | −1.156 |

$H_2O$ (a.u.):

| | | | |
|---|---|---|---|
| O | 0 | 0 | −0.1239093563 |
| H | 0 | 1.429937284 | 0.9832657567 |
| H | 0 | −1.429937284 | 0.9832657567 |

$NH_3$ (a.u.):

| | | | |
|---|---|---|---|
| N | 0 | 0 | −0.1277338768 |
| H | 0 | −1.7699234620 | 0.5915930938 |
| H | 1.532798681 | 0.8849617311 | 0.5915930938 |
| H | −1.532798681 | 0.8849617311 | 0.5915930938 |

*E-mail address: damatthews@smu.edu

CO (a.u.):

O 0 0 0.913973
C 0 0 −1.218243

## 2. Core Ionization Potentials

The first core ionization potentials are listed as absolute vertical energies for the CVS-EOM-CCSDT reference, and as relative errors ($E(X) - E(CCSDT)$) for all other methods. CVS-EOM-CC methods are listed in abbreviated form, e.g. "CCSDT" = CVS-EOM-CCSDT. For molecules with heterogeneous nuclei, the edge under consideration is indicated by an asterisk (the energies for $C_2H_4$ are the average of the gerade and ungerade combinations). The errors are summarized by the average error, $\bar{E}$, and the standard deviation, $\sigma$, used to construct the normal error distribution plots in the manuscript.

| | CCSDT | CC3 | CCSDT-3 | CCSDT-1 | CCSD |
|---|---|---|---|---|---|
| $C_2^*H_4$ | 290.804 | 0.054 | 0.46 | 0.019 | 1.432 |
| HCN* | 406.711 | -0.183 | 0.356 | -0.212 | 1.593 |
| HC*N | 293.532 | 0.129 | 0.443 | 0.178 | 1.082 |
| $H_2O^*$ | 539.464 | -0.734 | -0.025 | -0.62 | 1.939 |
| $N^*H_3$ | 405.466 | -0.298 | 0.198 | -0.292 | 1.565 |
| C*O | 296.431 | 0.099 | 0.422 | 0.343 | 1.189 |
| CO* | 542.255 | -0.687 | 0.086 | -0.612 | 2.014 |
| $\bar{E}$ | – | 0.231 | -0.277 | 0.171 | -1.545 |
| $\sigma$ | – | 0.335 | 0.178 | 0.345 | 0.323 |

| | CCSD* | CCSDR(3) | CCSD(T)(a)* | ΔCCSD | CCSD(T)(a) |
|---|---|---|---|---|---|
| $C_2H_4$ | 0.267 | 0.541 | 0.535 | – | 0.029 |
| HCN* | 0.208 | -0.401 | 0.589 | 0.073 | 0.071 |
| HC*N | 0.169 | 0.481 | 0.458 | -0.012 | 0.073 |
| $H_2O$ | 0.145 | 0.367 | 0.373 | 0.181 | 0.016 |
| $NH_3$ | 0.175 | 0.431 | 0.419 | 0.145 | 0.027 |
| C*O | 0.069 | 0.423 | 0.385 | 0.002 | 0.136 |
| CO* | 0.300 | 0.420 | 0.469 | 0.127 | -0.043 |
| $\bar{E}$ | -0.190 | -0.323 | -0.461 | -0.085 | -0.044 |
| $\sigma$ | 0.071 | 0.300 | 0.073 | 0.073 | 0.052 |

## 3. Vertical Excitation Energies

The first four vertical core excitation energies are given for each edge. The CVS-EOM-CCSDT energies are absolute, while relative errors ($E(X) - E(CCSDT)$) for all other methods. CVS-EOM-CC methods are listed in abbreviated form, e.g. "CCSDT" = CVS-EOM-CCSDT. For molecules with heterogeneous nuclei, the edge under consideration is indicated by an asterisk (the energies for $C_2H_4$ are the average of the gerade and ungerade combinations). The errors are summarized by the average error, $\bar{E}$, and the

standard deviation, $\sigma$, used to construct the normal error distribution plots in the manuscript.

| | | CCSDT | CC3 | CCSDT-3 | CCSDT-1 | CCSD |
|---|---|---|---|---|---|---|
| $C_2^*H_4$ | $K \to \pi^*$ | 285.081 | 0.236 | 0.399 | 0.234 | 1.022 |
| | $K \to 3s$ | 287.372 | 0.161 | 0.491 | 0.143 | 1.318 |
| | $K \to 3p$ | 288.014 | 0.154 | 0.484 | 0.137 | 1.316 |
| | $K \to 4p$ | 288.135 | 0.147 | 0.523 | 0.125 | 1.522 |
| $HCN^*$ | $K \to \pi^*$ | 400.029 | 0.149 | 0.360 | 0.086 | 1.073 |
| | $K \to 3s$ | 402.746 | -0.115 | 0.483 | -0.144 | 2.037 |
| | $K \to 4s$ | 403.209 | 0.020 | 0.464 | -0.016 | 1.613 |
| | $K \to 3p$ | 404.357 | -0.033 | 0.461 | -0.071 | 1.680 |
| $HC^*N$ | $K \to \pi^*$ | 286.824 | 0.183 | 0.317 | 0.287 | 0.713 |
| | $K \to 3s$ | 289.526 | 0.180 | 0.406 | 0.265 | 0.896 |
| | $K \to 4s$ | 290.070 | 0.207 | 0.467 | 0.269 | 1.041 |
| | $K \to 3p$ | 291.158 | 0.186 | 0.444 | 0.245 | 0.982 |
| $H_2O^*$ | $K \to 3s$ | 533.960 | -0.310 | 0.168 | -0.260 | 1.633 |
| | $K \to 3p$ | 535.780 | -0.360 | 0.134 | -0.308 | 1.591 |
| | $K \to 4s$ | 537.300 | -0.430 | 0.118 | -0.372 | 1.730 |
| | $K \to 4p$ | 537.390 | -0.350 | 0.150 | -0.323 | 1.670 |
| $N^*H_3$ | $K \to 3s$ | 400.764 | -0.055 | 0.299 | -0.062 | 1.365 |
| | $K \to 3p$ | 402.437 | -0.108 | 0.270 | -0.114 | 1.352 |
| | $K \to 4s$ | 403.567 | -0.073 | 0.283 | -0.100 | 1.336 |
| | $K \to 5s$ | 404.317 | -0.136 | 0.274 | -0.133 | 1.479 |
| $C^*O$ | $K \to \pi*$ | 287.664 | 0.134 | 0.229 | 0.429 | 0.518 |
| | $K \to 3s$ | 292.868 | 0.197 | 0.473 | 0.422 | 1.170 |
| | $K \to \pi^*/3d$ | 293.924 | 0.186 | 0.467 | 0.413 | 1.157 |
| | $K \to 4s$ | 294.122 | 0.172 | 0.452 | 0.409 | 1.136 |
| $CO^*$ | $K \to \pi*$ | 534.209 | -0.133 | 0.265 | -0.266 | 1.635 |
| | $K \to 3s$ | 538.782 | -0.407 | 0.235 | -0.361 | 1.869 |
| | $K \to \pi^*/3d$ | 539.877 | -0.490 | 0.217 | -0.422 | 2.047 |
| | $K \to 4s$ | 539.969 | -0.571 | 0.197 | -0.479 | 2.253 |
| $\bar{E}$ | | – | 0.045 | -0.340 | -0.001 | -1.398 |
| $\sigma$ | | – | 0.246 | 0.126 | 0.279 | 0.401 |

| | | CCSD* | CCSDR(3) | CCSD(T)(a)* | ΔCCSD | CCSD* corr. |
|---|---|---|---|---|---|---|
| $C_2^*H_4$ | $K \rightarrow \pi^*$ | 0.217 | 0.476 | 0.479 | – | -0.021 |
| | $K \rightarrow 3s$ | 0.303 | 0.558 | 0.557 | – | 0.065 |
| | $K \rightarrow 3p$ | 0.298 | 0.550 | 0.553 | – | 0.060 |
| | $K \rightarrow 4p$ | 0.319 | 0.590 | 0.589 | – | 0.081 |
| $HCN^*$ | $K \rightarrow \pi^*$ | 0.118 | 0.521 | 0.526 | -0.047 | -0.019 |
| | $K \rightarrow 3s$ | 0.531 | 0.935 | 1.061 | 0.038 | 0.394 |
| | $K \rightarrow 4s$ | 0.107 | 0.505 | 0.384 | – | -0.030 |
| | $K \rightarrow 3p$ | 0.285 | 0.682 | 0.680 | 0.187 | 0.148 |
| $HC^*N$ | $K \rightarrow \pi^*$ | 0.032 | 0.370 | 0.369 | -0.069 | -0.064 |
| | $K \rightarrow 3s$ | 0.154 | 0.408 | 0.394 | 0.014 | 0.058 |
| | $K \rightarrow 4s$ | 0.187 | 0.488 | 0.475 | – | 0.091 |
| | $K \rightarrow 3p$ | 0.171 | 0.459 | 0.444 | 0.056 | 0.075 |
| $H_2O^*$ | $K \rightarrow 3s$ | 0.211 | 0.438 | 0.443 | 0.157 | 0.082 |
| | $K \rightarrow 3p$ | 0.208 | 0.434 | 0.442 | 0.135 | 0.079 |
| | $K \rightarrow 4s$ | 0.192 | 0.419 | 0.425 | 0.168 | 0.063 |
| | $K \rightarrow 4p$ | 0.188 | 0.428 | 0.429 | 0.159 | 0.059 |
| $N^*H_3$ | $K \rightarrow 3s$ | 0.211 | 0.457 | 0.449 | 0.135 | 0.063 |
| | $K \rightarrow 3p$ | 0.209 | 0.450 | 0.449 | 0.118 | 0.061 |
| | $K \rightarrow 4s$ | 0.188 | 0.440 | 0.433 | – | 0.040 |
| | $K \rightarrow 5s$ | 0.203 | 0.447 | 0.442 | – | 0.055 |
| $C^*O$ | $K \rightarrow \pi*$ | -0.057 | 0.284 | 0.275 | 0.038 | 0.010 |
| | $K \rightarrow 3s$ | 0.120 | 0.486 | 0.460 | 0.041 | 0.187 |
| | $K \rightarrow \pi^*/3d$ | 0.121 | 0.465 | 0.437 | 0.075 | 0.188 |
| | $K \rightarrow 4s$ | 0.118 | 0.438 | 0.410 | – | 0.185 |
| $CO^*$ | $K \rightarrow \pi*$ | 0.222 | 0.513 | 0.532 | -0.049 | -0.121 |
| | $K \rightarrow 3s$ | 0.378 | 0.512 | 0.553 | 0.161 | 0.035 |
| | $K \rightarrow \pi^*/3d$ | 0.379 | 0.523 | 0.551 | 0.153 | 0.036 |
| | $K \rightarrow 4s$ | 0.380 | 0.520 | 0.554 | 0.123 | 0.037 |
| $\bar{E}$ | | -0.214 | -0.493 | -0.493 | -0.084 | -0.068 |
| $\sigma$ | | 0.116 | 0.111 | 0.135 | 0.079 | 0.093 |

## 4. Term Values

The term values corresponding to the first four vertical core excitation energies are given for each edge. The term values are defined as the relative energy of the excitation compared to the first core ionization potential. The CVS-EOM-CCSDT term values are absolute, while relative errors $(T(X) - T(CCSDT))$ for all other methods. CVS-EOM-CC methods are listed in abbreviated form, e.g. "CCSDT" = CVS-EOM-CCSDT. For molecules with heterogeneous nuclei, the edge under consideration is indicated by an asterisk (the energies for $C_2H_4$ are the average of the gerade and ungerade combinations). The errors are summarized by the average error, $\bar{E}$, and the standard deviation, $\sigma$, used to construct the normal error distribution plots in the manuscript.

| | | CCSDT | CC3 | CCSDT-3 | CCSDT-1 | CCSD |
|---|---|---|---|---|---|---|
| $C_2^*H_4$ | $K \rightarrow \pi^*$ | -5.723 | 0.182 | -0.061 | 0.215 | -0.410 |
| | $K \rightarrow 3s$ | -3.433 | 0.107 | 0.031 | 0.124 | -0.114 |
| | $K \rightarrow 3p$ | -2.790 | 0.100 | 0.024 | 0.118 | -0.116 |
| | $K \rightarrow 4p$ | -2.669 | 0.093 | 0.063 | 0.106 | 0.090 |
| $HCN^*$ | $K \rightarrow \pi^*$ | -6.682 | 0.332 | 0.004 | 0.298 | -0.520 |
| | $K \rightarrow 3s$ | -3.965 | 0.068 | 0.127 | 0.068 | 0.444 |
| | $K \rightarrow 4s$ | -3.502 | 0.203 | 0.108 | 0.196 | 0.020 |
| | $K \rightarrow 3p$ | -2.354 | 0.150 | 0.105 | 0.141 | 0.087 |
| $HC^*N$ | $K \rightarrow \pi^*$ | -6.708 | 0.054 | -0.126 | 0.109 | -0.369 |
| | $K \rightarrow 3s$ | -4.006 | 0.051 | -0.037 | 0.087 | -0.186 |
| | $K \rightarrow 4s$ | -3.462 | 0.078 | 0.024 | 0.091 | -0.041 |
| | $K \rightarrow 3p$ | -2.374 | 0.057 | 0.001 | 0.067 | -0.100 |
| $H_2O^*$ | $K \rightarrow 3s$ | -5.504 | 0.424 | 0.193 | 0.360 | -0.306 |
| | $K \rightarrow 3p$ | -3.684 | 0.374 | 0.159 | 0.312 | -0.348 |
| | $K \rightarrow 4s$ | -2.164 | 0.304 | 0.143 | 0.248 | -0.209 |
| | $K \rightarrow 4p$ | -2.074 | 0.384 | 0.175 | 0.297 | -0.269 |
| $N^*H_3$ | $K \rightarrow 3s$ | -4.702 | 0.243 | 0.101 | 0.230 | -0.200 |
| | $K \rightarrow 3p$ | -3.029 | 0.190 | 0.072 | 0.178 | -0.213 |
| | $K \rightarrow 4s$ | -1.899 | 0.225 | 0.085 | 0.192 | -0.229 |
| | $K \rightarrow 5s$ | -1.149 | 0.162 | 0.076 | 0.159 | -0.086 |
| $C^*O$ | $K \rightarrow \pi*$ | -8.767 | 0.035 | -0.193 | 0.086 | -0.671 |
| | $K \rightarrow 3s$ | -3.563 | 0.098 | 0.051 | 0.079 | -0.019 |
| | $K \rightarrow \pi^*/3d$ | -2.507 | 0.087 | 0.045 | 0.070 | -0.032 |
| | $K \rightarrow 4s$ | -2.309 | 0.073 | 0.030 | 0.066 | -0.053 |
| $CO^*$ | $K \rightarrow \pi*$ | -8.046 | 0.554 | 0.179 | 0.346 | -0.379 |
| | $K \rightarrow 3s$ | -3.473 | 0.280 | 0.149 | 0.251 | -0.145 |
| | $K \rightarrow \pi^*/3d$ | -2.378 | 0.197 | 0.131 | 0.190 | 0.033 |
| | $K \rightarrow 4s$ | -2.286 | 0.116 | 0.111 | 0.133 | 0.239 |
| $\bar{E}$ | | – | -0.186 | -0.063 | -0.172 | 0.146 |
| $\sigma$ | | – | 0.130 | 0.089 | 0.090 | 0.225 |

| | | CCSD* | CCSDR(3) | CCSD(T)(a)* | ΔCCSD |
|---|---|---|---|---|---|
| $C_2^*H_4$ | $K \to \pi^*$ | -0.050 | -0.065 | -0.056 | – |
| | $K \to 3s$ | 0.036 | 0.017 | 0.022 | – |
| | $K \to 3p$ | 0.031 | 0.009 | 0.018 | – |
| | $K \to 4p$ | 0.052 | 0.049 | 0.054 | – |
| $HCN^*$ | $K \to \pi^*$ | -0.090 | 0.922 | -0.063 | -0.119 |
| | $K \to 3s$ | 0.323 | 1.336 | 0.472 | -0.034 |
| | $K \to 4s$ | -0.101 | 0.906 | -0.205 | – |
| | $K \to 3p$ | 0.077 | 1.083 | 0.091 | 0.115 |
| $HC^*N$ | $K \to \pi^*$ | -0.137 | -0.111 | -0.089 | -0.050 |
| | $K \to 3s$ | -0.015 | -0.073 | -0.064 | 0.033 |
| | $K \to 4s$ | 0.018 | 0.007 | 0.017 | – |
| | $K \to 3p$ | 0.002 | -0.022 | -0.014 | 0.075 |
| $H_2O^*$ | $K \to 3s$ | 0.066 | 0.071 | 0.070 | -0.024 |
| | $K \to 3p$ | 0.063 | 0.067 | 0.069 | -0.046 |
| | $K \to 4s$ | 0.047 | 0.052 | 0.052 | -0.013 |
| | $K \to 4p$ | 0.043 | 0.061 | 0.056 | -0.022 |
| $N^*H_3$ | $K \to 3s$ | 0.036 | 0.026 | 0.030 | -0.009 |
| | $K \to 3p$ | 0.034 | 0.019 | 0.030 | -0.027 |
| | $K \to 4s$ | 0.013 | 0.009 | 0.014 | – |
| | $K \to 5s$ | 0.028 | 0.016 | 0.023 | – |
| $C^*O$ | $K \to \pi*$ | -0.126 | -0.139 | -0.110 | 0.035 |
| | $K \to 3s$ | 0.051 | 0.063 | 0.075 | 0.038 |
| | $K \to \pi^*/3d$ | 0.052 | 0.042 | 0.052 | 0.073 |
| | $K \to 4s$ | 0.049 | 0.015 | 0.025 | – |
| $CO^*$ | $K \to \pi*$ | -0.078 | 0.093 | 0.063 | -0.176 |
| | $K \to 3s$ | 0.078 | 0.092 | 0.084 | 0.033 |
| | $K \to \pi^*/3d$ | 0.079 | 0.103 | 0.082 | 0.026 |
| | $K \to 4s$ | 0.080 | 0.100 | 0.085 | -0.004 |
| $\bar{E}$ | | -0.024 | -0.170 | -0.032 | 0.005 |
| $\sigma$ | | 0.085 | 0.375 | 0.109 | 0.066 |
